# Supplementary material for: Differentially Private Releasing via Deep Generative Model (Technical Report)
Source: arXiv:1801.01594 source file (2018-03-25)
Supplement: Supplementary file 1 [file appendix.tex]

\subsection*{Appendix A: Privacy Accounting}

\begin{theorem}
	There exists constants $c_1$ and
	$c_2$ so that given sampling ratio
	$q = m/n$ and the number of steps $t$,
	for any $\epsilon < c_1 q^2 t$,
	Algorithm~1 in \cite{Abadi:2016:dpdl} is $(\epsilon,
	\delta)$--differential privacy for any
	$\delta > 0$ if we choose
	\begin{equation*}
		\sigma \ge c_2 \frac{q\sqrt{T\log(1 / \delta)}}
		{\epsilon}.
	\end{equation*}
\end{theorem}

\subsection*{Appendix B: Network Architectures}

\textbf{MNIST} $D$: input~-$(28, 28, 1)$ $\rightarrow$ Conv~
	(nb\_filter: 64, filter\_size: 5, strides: 2, activation: leaky\_relu)~-$(14, 14, 64) \rightarrow$
	Conv~(128, 5, 2, leaky\_relu)~-$(7, 7, 128) \rightarrow$
	Conv~(256, 5, 2, leaky\_relu)~-$(4, 4, 256) \rightarrow$
	FullyConnect~(output\_dim: 1, activation: identity)~-$(1)$ .
	$G$: random noises~-$(128) \rightarrow $
	FullyConnect~(4096, identity)~-$(4096)  \rightarrow$ -> BN+ReLU~-$(4096) \rightarrow$
	ConvTranspose~(nb\_filters: 128, strides: 2, activations: ReLU)~-$(8, 8, 128)  \rightarrow$
	Slicing~-$(7, 7, 128) \rightarrow$
	ConvTranspose~(nb\_filters: 256, strides: 2, activations: ReLU)~-$(14, 14, 64) \rightarrow$
	ConvTranspose~(nb\_filters: 256, strides: 2, activations: tanh)~-$(28, 28, 1)$.

\vspace{3pt}
\textbf{CelebA}. $D$: input~-$(48, 48, 3) \rightarrow$
	Conv~(128, 5, 2, leaky\_relu)~-$(24, 24, 128) \rightarrow$
	Conv~(256, 5, 2, leaky\_relu)~-$(12, 12, 256) \rightarrow$
	Conv~(512, 5, 2, leaky\_relu)~-$(6, 6, 512) \rightarrow$
	FullyConnect~(1, identity)~-$(1)$ .
	$G$: random noises~-$(128) \rightarrow $
	FullyConnect~(18432, identity)~-$(18432)  \rightarrow$
	Upsample Residual Block~(512, 5)~-$(12, 12, 512) \rightarrow $
	Upsample Residual Block~(256, 5)~-$(24, 24, 256) \rightarrow $
	Upsample Residual Block~(128, 5)~-$(48, 48, 128) \rightarrow $
	BN + ReLU~-$(48, 48, 128) \rightarrow$
	Conv~(3, 3, 1, tanh)~-$(48, 48, 3)$.

\vspace{3pt}
\textbf{LSUN}. $D$: input~-$(64, 64, 3) \rightarrow$
	Conv~(64, 5, 2, leaky\_relu)~-$(32, 32, 64) \rightarrow$
	Conv~(128, 5, 2, leaky\_relu)~-$(16, 16, 128) \rightarrow$
	Conv~(256, 5, 2, leaky\_relu)~-$(8, 8, 256) \rightarrow$
	Conv~(512, 5, 2, leaky\_relu)~-$(4, 4, 512) \rightarrow$
	FullyConnect~(1, identity)~-$(1)$ .
	$G$: random noises~-$(128) \rightarrow $
	FullyConnect~(8192, identity)~-$(8192)  \rightarrow$
	Upsample Residual Block~(512, 5)~-$(8, 8, 512) \rightarrow $
	Upsample Residual Block~(256, 5)~-$(16, 16, 256) \rightarrow $
	Upsample Residual Block~(128, 5)~-$(32, 32, 128) \rightarrow $
	Upsample Residual Block~(64, 5)~-$(64, 64, 64) \rightarrow $
	BN + ReLU~-$(64, 64, 64) \rightarrow$
	Conv~(3, 3, 1, tanh)~-$(64, 64, 3)$.

% \item [5.] Structure of \textit{Upsample Residual Block}~(nb\_filter: n, filter\_size: s).  It is a residual
% 	structure which may not present properly with the arrow symbols.
	% \begin{algorithm}
	% 	\myproc{Upsample Residual Block~(nb\_filter: $n$, filter\_size: $s$, input: $x$)}
	% 	{
	% 		$\bar{x} \gets Upsample Conv(n, 1, x) $ \;
	% 		$x \gets ReLU\left(BN\left(x \right) \right) $ \;
	% 		$x \gets Upsample Conv(n, s, x) $ \;
	% 		$x \gets ReLU\left( BN\left(x\right) \right)$ \;
	% 		$x \gets Conv(n, s, \text{strides: } 1, x)$ \;
	% 		\Return $x + \bar{x}$
	% 	}
    %
	% 	\myproc{Upsample Conv~(nb\_filter: $n$, filter\_size: $s$, input: $x$)}
	% 	{
	% 		$\text{cat} \gets $ tf.concat([x, x, x, x], axis=-1)  \tcp*{seems difficulty to describe it here.}
	% 		$x \gets $ tf.depth\_to\_space(x, 2) \tcp*{basically, it provides a pure convolutional way
	% 			for upsampling instead of pooling.}
	% 		\Return Conv(n, s, 1, x)
	% 	}
	% 	\caption{Two components}
	% 	\label{alg:upsampleresidual}
	% \end{algorithm}
